# Supplementary material for: Parallel-Learning of Invariant and Tempo-variant Attributes of Single-Lead Cardiac Signals: PLITA
Source: arXiv:2502.21162 source file (2025-02-28)
Supplement: Supplementary file 1 [file appendix.tex]

\section{Data Preprocessing} \label{app:data}
To ensure the complete reproducibility of this work, this section presents a detailed description of the preprocessing steps employed for the training and evaluation databases utilized in the proposed method.

\subsection{\ac{SHHS} Data Selection}
Only the subjects that appear in both recording cycles are used during the training procedure. This leads to 2643 subjects. ECG signals are extracted from the \ac{PSG} recordings. The quality of every 10 seconds-data strips has been evaluated with the algorithm proposed by Zhao and Zhang \cite{ecg_quality}. We use SHHS since it contains two records belonging to the same subject. This makes this specific database special, and this is the reason that it has been the only database used during the optimization.

\subsection{Icentia Data Selection}
Due to computational limited resources, only 5 out of the 50 segments provided for each subject are used for the model training. These segments have been selected randomly.
The quality of every 10 seconds-data strip has been evaluated with the algorithm proposed by Zhao and Zhang \cite{ecg_quality}. 

\subsection{Data cleaning}
In addition, all signals from the utilized datasets were resampled to a frequency of 100Hz. Then, a $5^{th}$ order Butterworth high-pass filter with a cutoff frequency of 0.5Hz was applied to eliminate any DC-offset and baseline wander. Finally, each dataset underwent normalization to achieve unit variance, ensuring that the signal samples belong to a $\mathcal{N}(0, 1)$ distribution. This normalization process aimed to mitigate variations in device amplifications that may have occurred during the data collection.

\section{Additional Ablation Study} \label{appendix:sie}

Although we have decided not to incorporate either the representation split nor $\mathcal{L}_{reg}$ components of \ac{SIE} method, we have assessed their potential impact on the downstream tasks. Table \ref{tab:abla_sie} reflects the results of this evaluation. It can be seen how the performance, especially when the split operation is applied, is significantly deteriorated. This result is aligned with our line of reasoning about why not split the representations for \ac{ECG} processing detailed in Section \ref{sec:two_projectors}.

\begin{table}[h]
\centering
\caption{Effect of the incorporation of \ac{SIE} components. The bold type indicates the proposed configuration. Trained on SHHS dataset.}
\vskip 0.05in
\resizebox{0.99 \columnwidth}{!}{%
\label{tab:abla_sie}
\begin{tabular}{cc|cc}
\hline
Split & $\mathcal{L}_{reg}$ & \begin{tabular}[c]{@{}c@{}}AFib\\ Accuracy (\%)\end{tabular} & \begin{tabular}[c]{@{}c@{}} Sleep Stages \\ 2 Classes Accuracy (\%)\end{tabular} \\ \hline
\xmark & \xmark & \textbf{80.7} & \textbf{75.3}\\
\cmark & \xmark & 75.7 & 71.2  \\
\xmark & \cmark & 80.3 & 74.1 \\
\cmark & \cmark & 76.8 & 73.1 \\ 
\hline
\end{tabular}}
\end{table}

\noindent As detailed in the main manuscript, DIVA does not use data augmentation techniques. We consider that the noise inherent in ECG recordings is sufficient to dispense with it. However, the incorporation of both signal-reverse operation and vertical flip, used in CLOCS as data augmentation, has been evaluated. In addition, the use of Euclidean distance instead of Cosine Similarity is also evaluated. 

\begin{table}[h]
\centering
\caption{Additional Ablation Study.  The bold type indicates the proposed configuration. All methods have been trained on SHHS dataset.}
\vskip 0.05in
\resizebox{\columnwidth}{!}{%
\label{tab:abla3}
\begin{tabular}{cc|cc}
\hline
\begin{tabular}[c]{@{}c@{}}Distance\\ Metric \end{tabular} & \begin{tabular}[c]{@{}c@{}}Data\\ Augmentation\end{tabular} & \begin{tabular}[c]{@{}c@{}}AFib\\ Accu (\%)\end{tabular} & \begin{tabular}[c]{@{}c@{}} Sleep Stages \\ 2 Classes Accu (\%)\end{tabular} \\ \hline
Cosine Similarity & \xmark & \textbf{80.7} & \textbf{75.3}\\
Euclidean & \xmark & 80.9 & 70.3\\
Cosine Similarity & \cmark & 78.9 & 71.5  \\
\hline
\end{tabular}}
\end{table}

\noindent Table \ref{tab:abla3} shows that for both configurations, the performance of the model deteriorates significantly, especially in Sleep Classification. \\

\noindent Although we do not have a reasoning as to why this deterioration occurs when using Euclidean Distance, we do have an intuition as to why when data augmentation is incorporated. Existing studies, such as \cite{siamese}, finds that the incorporation of data augmentation in \ac{SSL} for video analysis does not provide any benefits. In addition to that, the selection of data augmentation operations to use in computer vision is highly contrasted. However, in the \ac{ECG} processing field it is not the case. As a prove of it several recent works, such as \cite{data_aug_1, data_aug_2} have proposed new data augmentation techniques in recent times. We believe that the combination of both factors could explain this drop on the performance.

\section{Siamese Masked Autoencoders Implementation}
This section provides details of the implementation of the Siamese Masked Autoencoder method. It is a method that is originally designed for image processing and there are no existing studies for is optimal implementation for 1D signals. Therefore, we have studied different configurations for the hyperparameters required by the method, i.e. Masking Ratio and Input Sampling Gap. Table \ref{tab:siam_auto} shows the performance for different hyperparameter configurations. We have included in the evaluation the best-performing one. Furthermore, the decoder implementation maintains the same ratio size with respect to the encoder in alignment with the original paper, leading to 3 transformer blocks with a dimensionality of 64. Finally, the cross-self decoder configuration has been evaluated since it produces the best results according to the original work.

\begin{table*}[h]
\caption{Ablation for Siamese Masked Autoencoders}
\label{tab:siam_auto}
\resizebox{0.8\textwidth}{!}{%
\begin{tabular}{cc|cc|cc}
\cline{3-6}
\multicolumn{2}{c|}{}                  & \multicolumn{2}{c|}{Afib Classification} & \multicolumn{2}{c}{Sleep Stage Classification} \\ \hline
Masking Ratio & Input Sampling Gap (s) & Accu (\%)         & F1 Score (\%)        & Accu (\%)                 & AUC                \\ \hline
0.9           & (30, 150)              & 59.2              & 44.3                 & 71.0                      & 0.69                \\
\textbf{0.75} & \textbf{(30, 150)}     & \textbf{76.5}     & \textbf{73.0}        & \textbf{72.9}             & \textbf{0.74}         \\
0.5           & (30, 150)              & 71.9              & 67.1                 & 71.1                      & 0.73                 \\
0.75          & (10, 120)              & 75.9              & 71.6                 & 72.9                      & 0.75                 \\
0.75          & (60, 180)              & 76.1              & 72.7                 & 72.9                      & 0.74                \\ \hline
\end{tabular}}
\end{table*}

\newpage
\section{Comments about using AFib Identification for Dynamics Feature Exploration} \label{app:selection}

\noindent Subjects tend to be in a normal or AFib state for a long period of time. Therefore, we can imagine other subject-changes, such as different physical activities or changes in mental states, taking place with a higher frequency. Although the study of the tempo-variant features would have been optimal in these tasks, the absence of labeled data prompted the use of labeled AFIb datasets. Due to this, a selection of the records with the most state changes has been made. We only consider recordings for which the predominant label is present, at the most, in the 80\% of instances in the recording. It leads to using just 10 recordings. It is assumed that the tempo-variant attributes capable of explaining the differences between these states will have more variance in these selected records, so they will appear in the tempo-variant cluster. Figure \ref{fig:used} shows an example of a record that has been used while Figure \ref{fig:non-used} shows an example of a record that has not been used. \\

\begin{figure}[H]
\centering
\subfloat[Example of used record]
{\fbox{\includegraphics[width=\columnwidth]{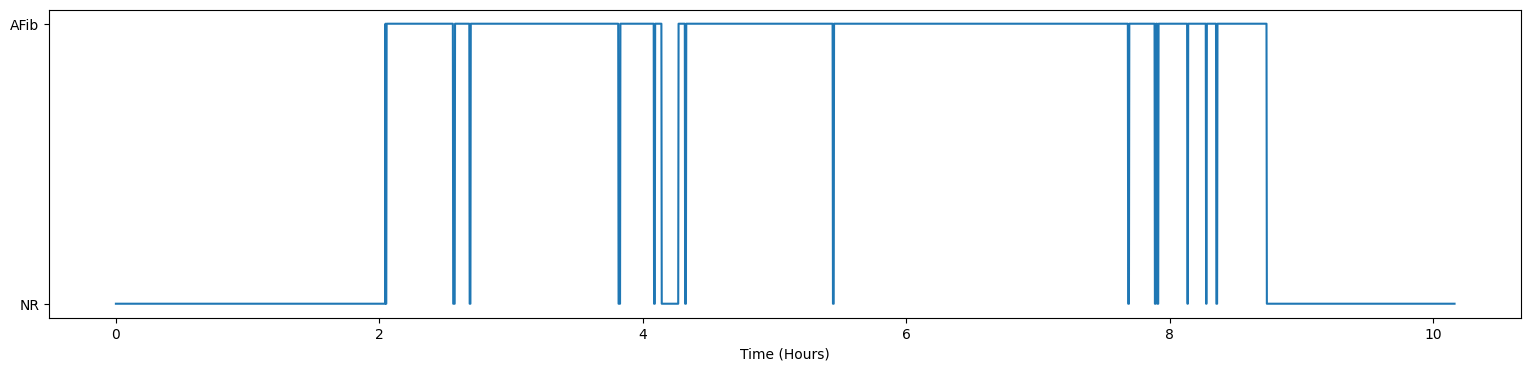}\label{fig:used}}}
\hfill
\subfloat[Example of non-used record]
{\fbox{\includegraphics[width=\columnwidth]{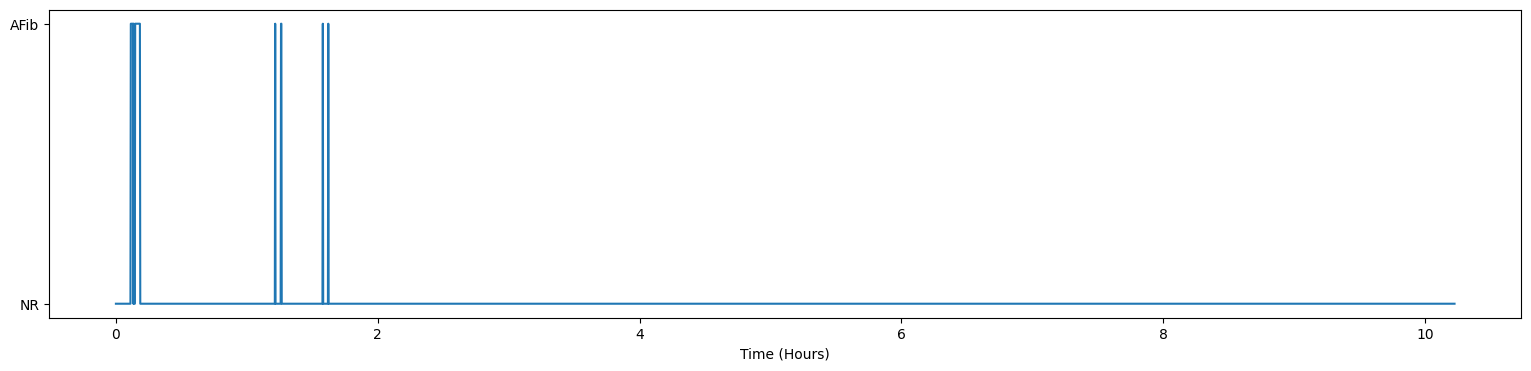}\label{fig:non-used}}}
\caption{\ac{MIT-AFIB} record selection}
\label{fig:afib_selection}
\end{figure}

\noindent This line of reasoning also explains why, although 3 of the 5 important features are contained in this set, as shown in Section \ref{sec_shap}, their overlapping ratio is not as significant as others contained within the tempo-variant sets.

\begin{algorithm*}
\SetAlgoLined
\KwIn{

    \\  \hspace{0.5cm} \textit{K} and \textit{B} \Comment{Number of iterations and Batch Size}
    \\  \hspace{0.5cm} $D^1$ and $D^2$ \Comment{Set of time series from Recordings 1 and 2}
    \\ \hspace{0.5cm} $\mathcal{F}(x)$ and $\mathcal{F\prime}(x)$ \Comment{Student Encoder and Teacher Encoder}
    \\ \hspace{0.5cm}  $\mathcal{G}(h)_{iv}$ and $\mathcal{G}(h)_{tv}$ \Comment{Student Invariant and Tempo-variant Projectors}
    \\ \hspace{0.5cm} $\mathcal{G\prime}(\eta)_{iv}$ and  $\mathcal{G\prime}(\eta)_{tv}$ \Comment{Teacher Invariant and Tempo-variant Projectors}
    \\ \hspace{0.5cm}  $\mathcal{Q}(z)_{iv}$ and $\mathcal{Q}(z)_{tv}$ \Comment{Student Invariant and Tempo-variant Predictors}
    
    \\ \hspace{0.5cm} $\theta$ , and $\xi$ \Comment{Student and Teacher Parameters}
    \\ \hspace{0.5cm} \textit{opt} and $\tau$ \Comment{Optimizer and EMA update parameter}
    %\\ \hspace{0.5cm} $\mathcal{PAR}$ \Comment{Ponderate Average Representation}
    \\ \hspace{0.5cm} $\mathcal{L}_{iv}$ and $\mathcal{L}_{tv}$ \Comment{Similarity and Gradual Loss Functions} 
    
    \\ \hspace{0.5cm} $W$ and $N$  \Comment{Windows Size, and \# Inputs per recording}}
    
\vspace{0.25cm}
\For{$k \gets 0$ \KwTo $K$}{
        $\mathcal{B} \gets {\{X_1^1 \cdots X_N^{1}, {X_1^2 \cdots X_N^{2}} \in D^1, D^2\}_{b = 0} ^ B}$ 
        \Comment{Sample $N$ inputs to form $X^1$ and $X^2$ from dataset} 
        \vspace{0.2cm}
        
        \For{$X^1, X^2 \in \mathcal{B}$}{
        \vspace{0.2cm}
        $h^1, h^2 \gets \mathcal{F}_(X^1,X^2)$ 
        \Comment{Student Encoder Representations for $X^1$ and $X^2$}

        $\eta^1, \eta^2 \gets \mathcal{F\prime}_(X^1, X^2)$ \Comment{Teacher Encoder Representations for $X^1$ and $X^2$}\\
        \vspace{0.2cm}
        
        $z^1_{iv}, z^2_{iv} \gets \mathcal{G}_{iv}(h^1, h^2)$ \Comment{Student Invariant Projections}

        $z^1_{tv},z^2_{tv} \gets \mathcal{G}_{tv}(h^1, h^2)$ \Comment{Student  Tempo-variant Projections}\\
        \vspace{0.2cm}
        
        $\upzeta^1_{iv}, \upzeta_{iv}^2 \gets \mathcal{G\prime}_{iv}(\eta^1, \eta^2)$ \Comment{Teacher Invariant Projections}
        
        $\upzeta^1_{tv}, \upzeta_{tv}^2 \gets \mathcal{G\prime}_{tv}(\eta^1, \eta^2)$ \Comment{Teacher Tempo-variant Projections}\\
        
        \vspace{0.2cm}
        
        $\mathbf{l}_n^{iv} \gets  0.5\cdot (\mathcal{L}_{iv}(\mathcal{Q}_{iv}(z^1_{iv}), \mathbf{\upzeta}^2_{iv}) + \mathcal{L}_{iv}(\mathcal{Q}_{iv}({z}^2_{iv}), \mathbf{\upzeta}^1_{iv})) $\Comment{Invariant Loss}

        \vspace{0.2cm}
        
       $\mathbf{l}_n^{tv} \gets  0.5\cdot (\mathcal{L}_{tv}(\mathcal{Q}_{tv}(z^1_{tv}), \mathbf{\upzeta}^1_{tv}) + \mathcal{L}_{tv}(\mathcal{Q}_{tv}({z}^2_{tv}), \mathbf{\upzeta}^2_{tv})) $\Comment{Tempo-variant Loss}
        \vspace{0.2cm}
    }
    \vspace{0.2cm}
    $\partial \theta \gets \sum_{b=0}^{B} (\partial_{\theta} \mathbf{l}_n^{iv} + \partial_{\theta} \mathbf{l}_n^{tv})$ \Comment{Compute loss gradients for $\theta$} \\

    \vspace{0.2cm}
    $\theta \gets \textit{opt}(\theta, \partial_{\theta})$ \Comment{Update Student Parameters}\\
    $\xi \leftarrow \tau \cdot \xi+(1-\tau) \cdot \theta$ \Comment{Update Teacher Parameters}
    }
\caption{\acf{PLITA}}
\label{algo}
\end{algorithm*}

\newpage
